# Supplementary material for: Time series classification for varying length series
Source: arXiv:1910.04341 source file (2019-10-10)
Supplement: Supplementary file 1 [file additional.tex]

\subsection{Identifying the most suitable processing technique}
	\label{subsec:best processor}
	Recall that one of our objectives is to identify the processing techniques that best fit a time series dataset generated from an underlying mechanism without any knowledge on the TSC algorithm.
	Hence, we perform further analysis on our results.
	We first compute the average accuracy for each of the processing technique and rank them using the same method as previous section. 
	In this case, with $k=5$ processing techniques, $N=85$ datasets, and critical value $q_{0.05}=2.728$, the average ranks have to be greater than a critical difference of $CD=0.6616$.
	
	The critical difference diagrams shown in Figures \ref{fig:cd plots for processors by generator} show the average ranks for each of the processing techniques. 
	First of all, the results show the importance of processing the time series to equal length as using time series with unequal length (No Processing and Prefix Suffix Zero) do not perform well for any of the mechanisms. 
	Figure \ref{fig:cd uniform processor} and \ref{fig:cd non uniform processor} show that re-scaling the time series to the same length outperforms other techniques for time series generated with fixed or varying frequencies.
	As suggested in the previous section, padding the prefix type time series (missing observations at the suffix) with random noise works well on average.
	This makes sense because by padding the suffix with random noise allows the algorithms to focus on the discriminating features in the prefix of the time series without introducing false features by re-scaling the time series.
	Similarly, for suffix and subsequence type time series, padding the prefix and suffix with noise works best but is not significantly different from re-scaling to the same length.
	
	\begin{figure}
	    \centering
	    \begin{subfigure}[]{\linewidth}
			\includegraphics[width=\linewidth]{images/cd_generators_processors/uniform_sampling.pdf}
			\caption{}
			\label{fig:cd uniform processor}
		\end{subfigure}
		\begin{subfigure}[]{\linewidth}
			\includegraphics[width=\linewidth]{images/cd_generators_processors/non_uniform_sampling.pdf}
			\caption{}
			\label{fig:cd non uniform processor}
		\end{subfigure}
		\begin{subfigure}[]{\linewidth}
			\includegraphics[width=\linewidth]{images/cd_generators_processors/prefix.pdf}
			\caption{}
			\label{fig:cd prefix processor}
		\end{subfigure}
		\hfill
		\begin{subfigure}[]{\linewidth}
			\includegraphics[width=\linewidth]{images/cd_generators_processors/suffix.pdf}
			\caption{}
			\label{fig:cd suffix processor}
		\end{subfigure}
		\begin{subfigure}[]{\linewidth}
			\includegraphics[width=\linewidth]{images/cd_generators_processors/subsequence.pdf}
			\caption{}
			\label{fig:cd subsequence processor}
		\end{subfigure}
		
	    \caption{The average ranking of the different processing techniques in terms of classification accuracy on datasets modified by (a) Uniform Sampling (b) Non Uniform Sampling (c) Prefix (d) Suffix (e) Subsequence mechanism.}
	    \label{fig:cd plots for processors by generator}
	\end{figure}
	
	\subsection{Identifying the most suitable classification algorithm}
	\label{subsec:best classifier}
	We perform a similar analysis as Section \ref{subsec:best processor} to identify the most suitable classification algorithm without having any knowledge on the processing techniques.
	In this case, we have $k=7$ classification algorithms, $N=85$ datasets and critical value $q_{0.05}=2.949$, giving a critical difference of $CD=0.9769$.
	
	Figures \ref{fig:cd plots for classifiers by generator} show the average ranks for each of the classification algorithms.
	Not surprisingly, the state-of-the-art ensemble algorithms perform really well on the different mechanisms with Proximity Forest being the most robust. 
	It is also expected that \nndtw{} performs really well on time series with variations in its frequencies relative to another time series. 
	However, it is disappointing to see that the algorithms that are capable of handling variable lengths in the literature such as Sliding Euclidean distance and Uniform Scaling with Euclidean distance did not perform so well. 
	The reason is that these methods are based on the Euclidean distance.
	So, even if they are able to find the best position for the shorter time series to match the longer time series, they are unable to align the features of the two time series. 
	One possible improvement could be to use Uniform Scaling with \dtw{} \citep{fu2008scaling} which will yield similar results as \dtw{}. 
	
	\begin{figure}
	    \centering
	    \begin{subfigure}[]{\linewidth}
			\includegraphics[width=\linewidth]{images/cd_generators_classifiers/uniform_sampling.pdf}
			\caption{}
			\label{fig:cd uniform classifier}
		\end{subfigure}
		\begin{subfigure}[]{\linewidth}
			\includegraphics[width=\linewidth]{images/cd_generators_classifiers/non_uniform_sampling.pdf}
			\caption{}
			\label{fig:cd non uniform classifier}
		\end{subfigure}
		\begin{subfigure}[]{\linewidth}
			\includegraphics[width=\linewidth]{images/cd_generators_classifiers/prefix.pdf}
			\caption{}
			\label{fig:cd prefix classifier}
		\end{subfigure}
		\hfill
		\begin{subfigure}[]{\linewidth}
			\includegraphics[width=\linewidth]{images/cd_generators_classifiers/suffix.pdf}
			\caption{}
			\label{fig:cd suffix classifier}
		\end{subfigure}
		\begin{subfigure}[]{\linewidth}
			\includegraphics[width=\linewidth]{images/cd_generators_classifiers/subsequence.pdf}
			\caption{}
			\label{fig:cd subsequence classifier}
		\end{subfigure}
		
	    \caption{The average ranking of the different classifiers in terms of classification accuracy on datasets modified by (a) Uniform Sampling (b) Non Uniform Sampling (c) Prefix (d) Suffix (e) Subsequence mechanism.}
	    \label{fig:cd plots for classifiers by generator}
	\end{figure}
	
	\subsection{Identifying the most suitable processing technique for a given classification algorithm}
	\label{subsec:limited resources}
	Finding the most suitable classification algorithm for each mechanism is important, but in many scenarios, the choice of a classification algorithm is limited by computational resources. 
	Hence, we further extend our analysis by assuming that we know the underlying mechanisms of our time series data and we would like to know which processing technique will give the best performance for a particular classification algorithm. 
	
	Using the classification accuracy results from Section \ref{subsec:overall results}, for each mechanism and classifier, we rank the processing techniques and compute the average ranks across all $N=85$ datasets.
	As the ensemble-based algorithms are unable to handle variable lengths time series, they are only evaluated on the three processing techniques mentioned in Section \ref{subsec:evaluation}. 
	
	Table \ref{tab:average rankings} shows the average ranks of each classification algorithm paired with a processing technique on the respective mechanism.
	Re-scaling the time series to the same length works best for datasets generated with varying frequencies regardless of the algorithm used.
	This makes sense because if the frequency of a time series is a fixed ratio relative to the other time series, then surely the best way is to re-scale them so that they have the same frequency.
	This confirms the results obtained in Section \ref{subsec:best processor}.
	
	For prefix type datasets, padding suffixes with noise perform well for algorithms that uses Euclidean distance, including \pf{}.
	Adding a single zero to the prefix and suffix works best for \nndtw{} and \nnsbd{}. 
	\boss{} performs best after the prefix and suffix of the time series are padded with noise.
	However, for suffix type datasets, re-scaling the time series to equal length performs the best for Euclidean distance algorithms and \pf{}.
	\nndtw{} still performs best when a single zero is added to the prefix and suffix of the time series.
	\boss{} and \nnsbd{} works best by padding the suffix with noise.
	All the techniques except re-scaling are not significantly different for \nnsbd{} suggests that \nnsbd{} is robust when dealing with such mechanisms.
	
	For subsequence type datasets, noise padding and re-scaling works well on Euclidean distance algorithms.
	\nndtw{} performs best with noise padded to the prefix and suffix of the subsequence because this will give better alignment of the features in both time series.
	Similar to other mechanisms, there are no significant difference between the processing techniques except re-scaling to the same length for \nnsbd{}.
	For the state of the arts, \boss{} works best with noise padding while \pf{} works best with re-scaling.  
	
	\begin{table}[]
	    \centering
	    \begin{tabular}{|c|c|c|c|c|c|c|}
	    \hline
	    TSC Algorithms & \rotatebox{90}{No Processing} &  \rotatebox{90}{Prefix Suffix Zero} & \rotatebox{90}{Prefix Suffix Noise}& \rotatebox{90}{Suffix Noise} & \rotatebox{90}{Re-scale} \\ \hline
	    \multicolumn{6}{|c|}{Uniform Sampling} \\ \hline
	    \nned{} & 4.259	& 3.894 & 2.718 & 2.747 & \textbf{1.382} \\
	    \nndtw{} & 2.804 & 2.709 & 3.981 & 3.734 & \textbf{1.772} \\
	    \nned{}-\textsc{Sliding} & 4.141 & 3.924 & 2.618 & 2.918 & \textbf{1.400}  \\
	    \nnus{} & 3.872 & 4.030 & 3.207 & 2.323 & \textbf{1.567} \\
	    \nnsbd{} & 3.444 & 3.444 & 3.250 & 3.438 & \textbf{1.425} \\
	    \boss{} & - & - & 2.462 & 2.481 & \textbf{1.057} \\
	    \pf{} & - & - & 2.318 & 2.534 & \textbf{1.149} \\
	    \hline
	    \multicolumn{6}{|c|}{Non Uniform Sampling} \\ \hline
	    \nned{} & 3.418	& 3.365 & 3.353 & 3.035 & \textbf{1.829} \\
	    \nndtw{} & 2.870 & 2.938 & 3.171 & 3.233 & \textbf{2.788} \\
	    \nned{}-\textsc{Sliding} & 3.147 & 3.206 & 3.371 & 3.206 & \textbf{2.071} \\
	    \nnus{} & 2.854 & 3.120 & 3.722 & 2.867 & \textbf{2.437} \\
	    \nnsbd{} & 3.316 & 3.316 & 3.319 & 3.289 & \textbf{1.763} \\
	    \boss{} & - & - & 2.205 & 2.280 & \textbf{1.515} \\
	    \pf{} & - & - & 1.938 & 2.322 & \textbf{1.740} \\
	    \hline
	    \multicolumn{6}{|c|}{Prefix} \\ \hline
	    \nned{} & 3.818	& 3.276 & 2.235 & \textbf{2.224} & 3.447 \\
	    \nndtw{} & 3.167 & \textbf{2.587} & 3.280 & 2.893 & 3.073 \\
	    \nned{}-\textsc{Sliding} & 4.041 & 3.382 & 2.959 & \textbf{1.776} & 2.841 \\
	    \nnus{} & & & & & \\
	    \nnsbd{} & \textbf{2.625} & \textbf{2.625} & 2.743 & 2.757 & 4.250 \\
	    \boss{} & - & - & \textbf{1.545} & 2.032 & 2.423 \\
	    \pf{} & - & - & 2.308 & \textbf{1.425} & 2.267 \\
	    \hline
	    \multicolumn{6}{|c|}{Suffix} \\ \hline
	    \nned{} & 3.835	& 3.906 & 2.659 & 2.653 & \textbf{1.947} \\
	    \nndtw{} & 3.147 & \textbf{2.353} & 2.680 & 3.747 & 3.073 \\
	    \nned{}-\textsc{Sliding} & 3.165 & 2.694 & 3.700 & 3.700 & \textbf{1.741} \\
	    \nnus{} & & & & & \\
	    \nnsbd{} & 2.809 & 2.809 & 2.724 & \textbf{2.651} & 4.007 \\
	    \boss{} & - & - & 1.936 & \textbf{1.571} & 2.494 \\
	    \pf{} & - & - & 1.921 & 2.264 & \textbf{1.814} \\
	    \hline
	    \multicolumn{6}{|c|}{Subsequence} \\ \hline
	    \nned{} & 3.982	& 3.765 & 2.412 & \textbf{2.382} & 2.459 \\
	    \nndtw{} & 3.473 & 2.867 & \textbf{2.393} & 3.440 & 2.827 \\
	    \nned{}-\textsc{Sliding} & 3.582 & 3.876 & \textbf{2.318} & 2.588 & 2.635 \\
	    \nnus{} & & & & & \\
	    \nnsbd{} & \textbf{2.684} & \textbf{2.684} & 2.757 & 2.737 & 4.138 \\
	    \boss{} & - & - & 1.885 & \textbf{1.776} & 2.340 \\
	    \pf{} & - & - & 2.007 & 2.158 & \textbf{1.836} \\
	    \hline
	    \end{tabular}
	    \caption{Average rankings of each of the classification algorithm paired with a processing technique on the respective mechanism.}
	    \label{tab:average rankings}
	\end{table}
